# Supplementary material for: Single-shot ToF sensing with sub-mm precision using conventional CMOS sensors
Source: arXiv:2212.00928 ancillary file (2022-12-02)
Supplement: Supplementary file 1 [file supplemental.pdf]

# Supplementary Material for: Single-shot ToF sensing with sub-mm precision using conventional CMOS sensors

**Manuel Ballester[1,*], Heming Wang[2,*], Jiren Li[2], Oliver Cossairt[1,2], and Florian Willomitzer[3,**]**

[1]Department of Computer Sciences, Northwestern University, Evanston, IL 60208
[2]Department of Electrical and Computer Engineering, Northwestern University, Evanston, IL 60208

[3]Wyant College of Optical Sciences, University of Arizona, Tucson, AZ 85721

[*]Joint first authorship
[**]Correspondence: fwillomitzer@arizona.edu

## 1. Demodulation algorithm.

In this supplementary section, we will describe in detail how to retrieve the optical fields $E(\lambda_1)$ and $E(\lambda_2)$ from a single captured image $I(x,y)$. In the supp. sec. A, we will provide some mathematical background, defining the object and reference beams that arrive at the sensor. Then, supp. sec. B will explain the Fourier-based demodulation algorithm that recovers the optical fields.

### A. Mathematical background.

As mentioned in section 3.1 of the main paper, our setup has two reference sources that point directly towards the sensor array. One reference beam at $\lambda_1$ encloses an angle $\theta_1$ with the horizontal x-axis, while the other reference beam at $\lambda_2$ encloses an angle $\theta_2$ with the vertical y-axis of the detector. In addition, there is an object source that emits light beams at $\lambda_1$ and $\lambda_2$ to illuminate the object uniformly. The schematic of our setup is shown in supp. fig. 1 of the main paper, and our full setup including diagram of the illumination engine is shown in supp. fig. 2.

The light scattered off the object arrives at the sensor plane (at $z = z_0$) and was denoted as

$$E(\lambda_1) \equiv E_1(x,y;t)$$

$$E(\lambda_2) \equiv E_2(x,y;t) \quad \textbf{(1)}$$

We have adopted the right-hand side notation from Eq. 1 during this Supplementary Material to point out explicitly that the optical fields are depicted as 2D numerical arrays in $(x,y)$ and are also time-dependent. A similar notation extends to other variables. For instance, the *time-invariant* optical phasemap at $\lambda_1$ is represented as $\phi(\lambda_1) \equiv \phi_1(x,y)$.

<u>Object fields and reference fields:</u>

The reference beams propagate as spherical waves from their point sources (the end of the optical fibers) toward the sensor chip. The distance from the reference sources to the sensor location is relatively long (about 30 cm) compared to the sensor size (about 2.5 cm). Therefore, one can reasonably assume that the reference beam wavefront is almost planar at the sensor location. We modeled these beams as planar waves hitting the sensor with an offset angle. Thus, the electric fields $E_1^{\text{ref}}(x,y,t)$ and $E_2^{\text{ref}}(x,y,t)$ of both reference beams can then be described as

$$E_1^{\text{ref}}(x,y,t) = \frac{1}{2}|E_1^{\text{ref}}| \exp\{i(\omega_1 t - \boldsymbol{k_1}\cdot\boldsymbol{r} + \sigma_1)\} + cc$$

$$E_2^{\text{ref}}(x,y,t) = \frac{1}{2}|E_2^{\text{ref}}| \exp\{i(\omega_2 t - \boldsymbol{k_2}\cdot\boldsymbol{r} + \sigma_2)\} + cc \quad \textbf{(2)}$$

Here $cc$ denotes the complex conjugate of the previous term, which ensures that the reference fields are $real$ in nature. This common complex notation [1] is employed to ease future calculations. The field $E_1^{\text{ref}}(x,y,t)$ denotes the horizontal reference field at $\lambda_1$, and has the approximately constant amplitude $|E_1^{\text{ref}}|$ at the sensor plane location $(z = z_0)$. Moreover, $\omega_1 = 2\pi\, c/\lambda_1$ is the angular frequency ($c$ being the speed of light), and $\boldsymbol{k_1} = (k_1^x, k_1^y, k_1^z)$ is the so-called "propagation vector" that indicates the three-dimensional propagation direction of the planar wave [2]. The constant shift $\sigma_1$ denotes the initial phase. It is known that $|\boldsymbol{k_1}| = k_1 = 2\pi/\lambda_1$ and $\boldsymbol{k_1}\cdot\boldsymbol{r} = (k_1^x, k_1^y, k_1^z)\cdot(x,y,z=z_0)$ is the usual dot product. The light beam is unpolarized.

Considering the angle of the reference beams with respect to the optical axis ($\theta_1$ and $\theta_2$), we express the propagation vectors as $\boldsymbol{k_1} = (k_1\sin(\theta_1), 0, k_1\cos(\theta_1))$ and $\boldsymbol{k_2} = (0, k_2\sin(\theta_2), k_2\cos(\theta_2))$. Therefore, the reference beams become

$$E_1^{\text{ref}}(x,y,t) = \frac{1}{2}|E_1^{\text{ref}}| \exp\{i(\omega_1 t - k_1\cos(\theta_1) z_0 + \sigma_1 - k_1\sin(\theta_1)x)\} + cc$$

$$E_2^{\text{ref}}(x,y,t) = \frac{1}{2}|E_2^{\text{ref}}| \exp\{i(\omega_2 t - k_2\cos(\theta_2) z_0 + \sigma_2 - k_2\sin(\theta_2)y)\} + cc \quad \textbf{(3)}$$

Please note that $(k_1\cos(\theta_1)z_0 + \sigma_1)$ and $(k_2\cos(\theta_2)z_0 + \sigma_2)$ are just constant shift phases that do not change the phase difference for different positions $(x,y)$. Therefore, we can virtually neglect these terms.

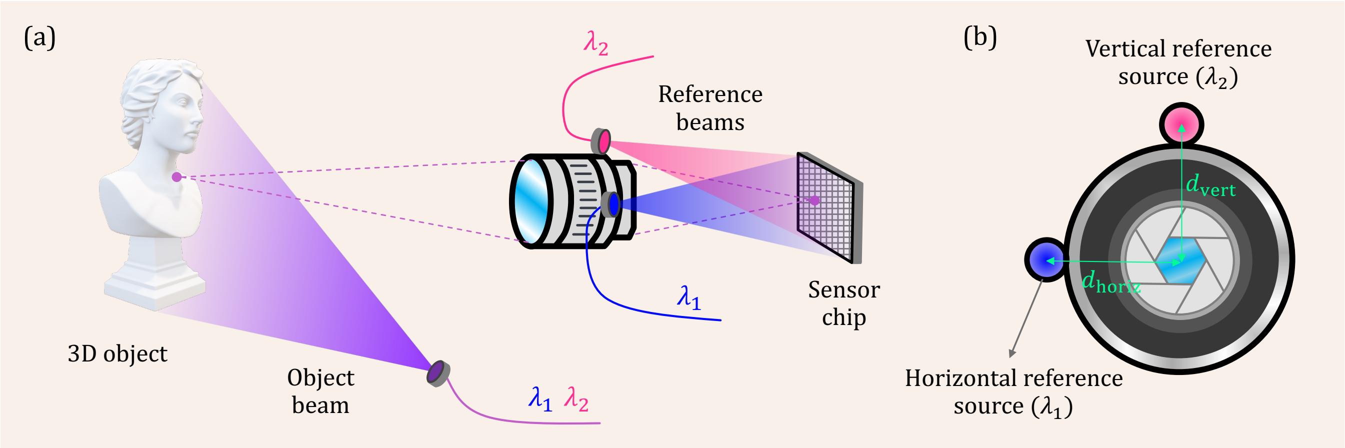


**Fig. 1.** Setup diagram for the novel camera based on the synthetic wavelength concept. (a) The 3D object is illuminated with an object beam that contains light waves at wavelengths $\lambda_1$ and $\lambda_2$. The field reflected in the object will pass through an imaging system and reach the camera sensor chip. In addition, two reference beams directly illuminate the sensor. (b) The frontal view of the optical system: Looking at the objective from the sensor location. The horizontal reference uses wavelength $\lambda_1$ and vertical reference $\lambda_2$. We control the angle at which the reference beams reach the sensor by modifying the distances $d_{\text{hor}}$ and $d_{\text{vert}}$.

In analogy to above, we can express the two object beams at $\lambda_1$ and $\lambda_2$ with the following general expressions:

$$E_1(x,y,t) = \frac{1}{2}|E_1(x,y)|\exp\{i(\omega_1 t - \phi_1(x,y))\} + cc$$

$$E_2(x,y,t) = \frac{1}{2}|E_2(x,y)|\exp\{i(\omega_2 t - \phi_2(x,y))\} + cc \quad \textbf{(4)}$$

The functions $\phi_1(x,y)$ and $\phi_2(x,y)$ denote the unknown phasemaps we want to retrieve. For optically rough surfaces, the optical phasemaps are “speckled”, i.e., they are complicated functions that are influences by the microscopic depth variation of the surface. Their also unknown amplitudes are represented by $|E_1(x,y)|$ and $|E_2(x,y)|$.

Intensity at the sensor location:
Four electric fields arrive at the sensor, two of them ($E_1$ and $E_2$) corresponding to the object beam and two ($E_1^{\text{ref}}$ and $E_2^{\text{ref}}$) corresponding to the reference beams. The intensity field at the sensor location is then

$$I \propto |E_1^{\text{ref}} + E_2^{\text{ref}} + E_1 + E_2|^2 \quad \textbf{(5)}$$

When we calculate the squared norm from Eq. 5, we find several interferences terms coming from the superposition of the different waves at different wavelengths. However, some of these terms corresponds to time-dependent interference fringes that oscillate too fast to be temporally resolved with a conventional sensor. As we are only interested in static interference fringes, we integrate over the sensor's exposure time, and the rapidly oscillating fringes average out. We collect these terms in the function $O(\lambda_1,\lambda_2) \approx 0$. For instance, these terms appear when we consider the superposition of waves with slightly different wavelengths, such as with the pairs $(E_1,E_2)$, $(E_1^{\text{ref}},E_2^{\text{ref}})$, $(E_1^{\text{ref}},E_2)$, and $(E_1,E_2^{\text{ref}})$. Supp. sec. 2 provides more information about these time-oscillating fringes and studies the interferences between the object beams, i.e., the particular case $(E_1,E_2)$.

In contrast, the interference between waves with the same wavelengths, such as the pairs $(E_1^{\text{ref}},E_1)$ and $(E_2^{\text{ref}},E_2)$, generate some fringes constant in time that the detector can resolve. These are the fringes we consider to analyze the intensity at the sensor location. Considering these comments, we can express Eq. 5 using Eqs. 3-4 as follows:

$$I(x,y) \propto |E_1^{\text{ref}}(x,y) + E_2^{\text{ref}}(x,y) + E_1(x,y) + E_2(x,y)|^2$$

$$= \frac{|E_1^{\text{ref}}|^2}{2} + \frac{|E_2^{\text{ref}}|^2}{2} + \frac{|E_1(x,y)|^2}{2} + \frac{|E_2(x,y)|^2}{2} + O(\lambda_1,\lambda_2)$$

$$+|E_1^{\text{ref}}||E_1(x,y)|\cos(\phi_1(x,y) - k_1\sin(\theta_1)x)$$

$$+|E_2^{\text{ref}}||E_2(x,y)|\cos(\phi_2(x,y) - k_2\sin(\theta_2)y) \quad \textbf{(6)}$$

We can rewrite Eq. 6 in a simpler form. First, we define the DC term:

$$a(x,y) = |E_1^{\text{ref}}|^2 + |E_2^{\text{ref}}|^2 + |E_1(x,y)|^2 + |E_2(x,y)|^2 \quad \textbf{(7)}$$

Then, the amplitudes of the static interference fringes can be denoted as

$$b_1(x,y) = |E_1^{\text{ref}}||E_1(x,y)|$$

$$b_2(x,y) = |E_2^{\text{ref}}||E_2(x,y)| \quad \textbf{(8)}$$

Finally, we establish $k_i\sin(\theta_i)2\pi f_i$, where $f_i$ are the so-called spatial carrier frequencies for $i \in \{1,2\}$. Then, we can re-formulate Eq. 6 using Eqs. 7-8 and setting $O(\lambda_1,\lambda_2) \approx 0$:

$$I(x,y) \propto a(x,y) + b_1(x,y)\cos(\phi_1(x,y) + 2\pi f_1 x)$$

$$+b_2(x,y)\cos(\phi_2(x,y) + 2\pi f_2 y) \quad \textbf{(9)}$$

Eq. 9 contains all the information about the experimental image $I(x,y)$ captured with our single-shot camera. The image $I(x,y)$ presents a speckle pattern overlayed with crossed interference fringes. The vertical fringes have a spatial carrier frequency $f_1$ in the x-axis; they are due to the interferences of the object beam $E_1(x,y)$ and the horizontal reference beam (at $\lambda_1$). Similarly, the horizontal fringes have a carrier frequency $f_2$ in the y-axis and occur from the interferences of the object beam $E_2(x,y)$ and the vertical reference beam (at

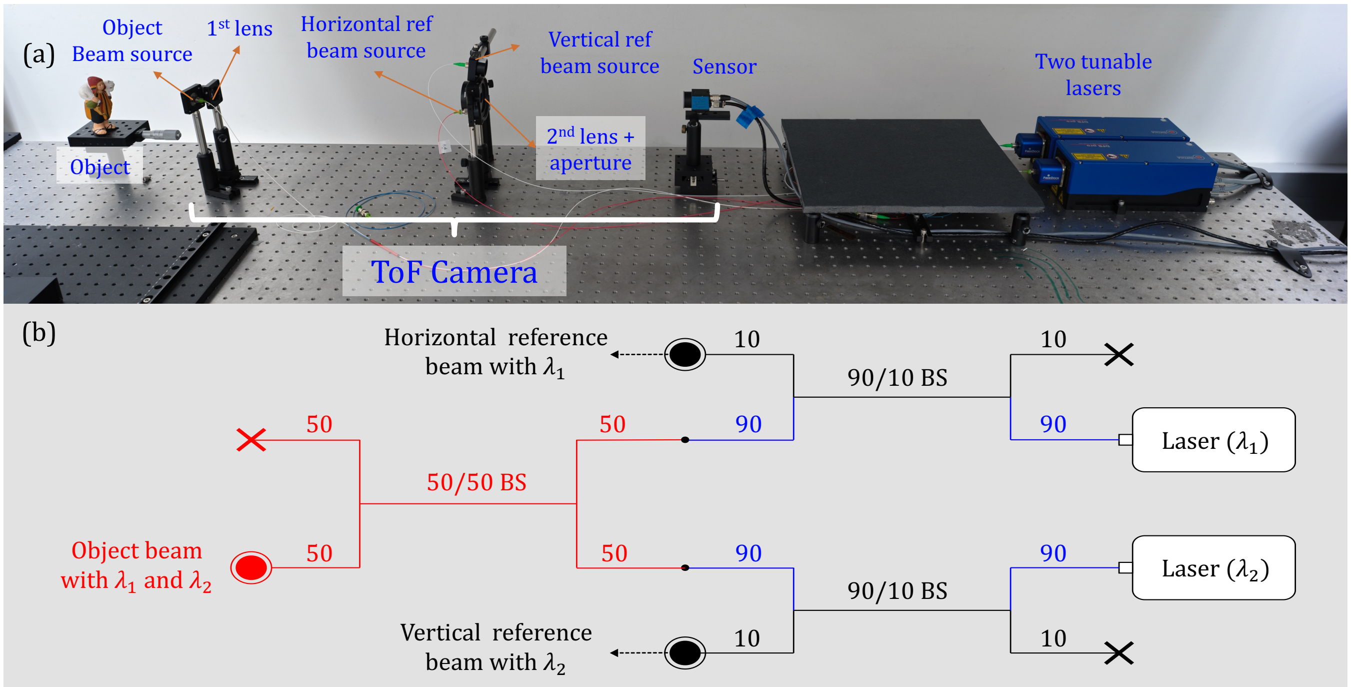


**Fig. 2.** (a) Photograph of our particular setup. Two identical tunable lasers will emit light in the NIR range at around 850 nm. We use optical fibers and beam splitters (BS) to direct the beams flexibly. We employ a 4f-system to image the object into the sensor array. (b) Diagram of the illumination engine.

$\lambda_2$). Supp. fig. 3 shows a original captured image and two zoom-in windows. In the first zoom-in window (supp. fig. 3 b), we can see the speckle pattern produced by the object beams. In the second zoom-in window (supp. fig. 3 c), we can nicely see the cross-like static fringes due to the interference between the object and the reference beams.

Our goal now is to retrieve the phases $\phi_1(x,y)$ and $\phi_2(x,y)$ from Eq. 6 known only the *real* numerical 2D array $I(x,y)$. Supp. sec. B will detail the demodulation algorithm for such a purpose.

## B. Demodulation algorithm.

Takeda *et al.* [3] proposed a technique to retrieve one phasemap using a Fourier-based demodulation algorithm. Similar demodulation procedures have been used in off-axis holography, interferometry, or fringe projection profilometry [4–9]. Our algorithm is inspired by this procedure and extended to the case of two phasemaps for applications in Computer Vision. Following the argument from [3], we define the following variables:

$$c_1(x,y) = \frac{1}{2} b_1(x,y) e^{i\phi_1(x,y)}$$

$$c_2(x,y) = \frac{1}{2} b_2(x,y) e^{i\phi_2(x,y)} \quad \textbf{(10)}$$

Then, we rewrite Eq. 9 using the definition of the complex cosine:

$$I(x,y) = a(x,y) + c_1(x,y)e^{i(2\pi f_1 x)} + c_1^*(x,y)e^{-i(2\pi f_1 x)}$$
$$+ c_2(x,y)e^{i(2\pi f_2 y)} + c_2^*(x,y)e^{-i(2\pi f_2 y)} \quad \textbf{(11)}$$

The 2D Fourier transform of the captured image $I(x,y)$ has then the following mathematical expression:

$$F[I](f_x,f_y) = A(f_x,f_y) + C_1(f_x - f_1, f_y) + C_1^*(f_x + f_1, f_y)$$
$$+ C_2(f_x, f_y - f_2) + C_2^*(f_x, f_y + f_2) \quad \textbf{(12)}$$

Where the capital letters denote the Fourier transform. We have employed the *linearity* and *shifting* properties of the Fourier transform [10] to derive Eq. 12 from 11. Please note that each function $(A, C_1, C_1^*, C_2, C_2^*)$ corresponds to the circular spectral region from supp. fig. 4a. As explained in section 4 of the main paper, we carefully adjusted the aperture size in the setup so that these regions do not overlap. Therefore, we can effectively crop out each region in the Fourier transform $F[I](f_x,f_y)$ of our experimental data.

We can follow the steps described in section 2.2 of the main paper to crop the horizontal region (the right-side one), corresponding to the term $C_1(f_x - f_1, f_y)$. First, we estimate the spatial carrier frequency $f_1$ as the center of the right-side spectral region. Then, we shift the spectrum using that carrier frequency so that $f_1$ is mapped right to the center of the Fourier transform (see supp. fig. 4b). Later, we apply a Hanning (or Gaussian) filter that effectively removes any other signals (see supp. fig. 4c). We have then successfully cropped the horizontal spectral region, $F_{\text{hor}}[I(x,y)] = C_1(f_x,f_y)$. If we calculate the inverse Fourier transform of the crop region using Eq. 10, we get the following:

$$\mathrm{F}^{-1}\{F_{\text{hor}}[I(x,y)]\} = c_1(x,y) = \tfrac{1}{2} b_1(x,y) e^{i\phi_1(x,y)} \quad \textbf{(13)}$$

Moreover, we know that $b_1(x,y) = |E_1^{\text{ref}}||E_1(x,y)|$ from Eq. 8. Thus, we find Eq. 3 from the main paper:

$$\mathrm{F}^{-1}\{F_{\text{hor}}[I(x,y)]\} \propto |E_1(x,y)| e^{i\phi_1(x,y)} = E_1(x,y) \quad \textbf{(14)}$$

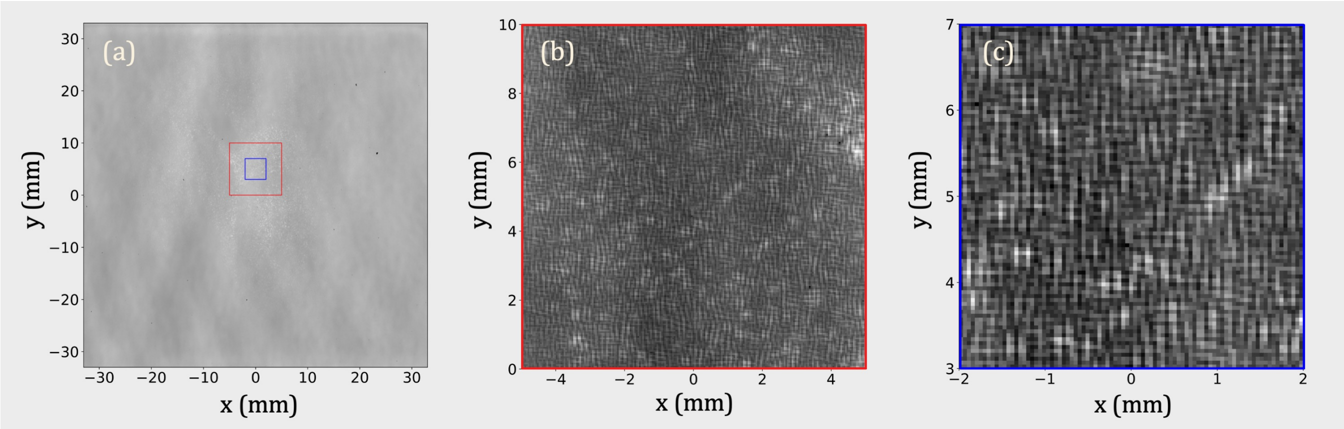


**Fig. 3.** (a) Image captured with our camera sensor. The spatial FoV of the camera is around 66mm × 66mm and the pixel resolution of the captured images is 1448×1448 pixels. We have cropped a window in the image at the central location pixels so that one can clearly see (b) the speckles (red window) and (c) the crossed vertical and horizontal fringes (blue window). The distance between fringes is about 3 pixels, near the sampling limit.

We have then easily recovered the speckle object field $E_1(x,y) \equiv E(\lambda_1)$. A similar procedure cropping the vertical region $C_2(f_x, f_y - f_2)$ leads to $E(\lambda_2)$.

Supp. fig. 5 (a,b,c,d) shows the absolute amplitudes and the phases at each optical wavelength. We can observe the speckle pattern in the amplitude images (supp. fig. 5 a,c) and the randomized phases in supp. fig. 5 b,d.

## 2. Synthetic Wavelength Interferometry.

The demodulation algorithm allowed us to recover the complex fields scattered off the object's surface at the optical wavelengths. In complex notation, these waves can be represented as:

$$E_1(x,y,t) = \frac{1}{2}|E_1(x,y)|\exp\{i(\omega_1 t - \phi_1(x,y))\} + cc$$

$$E_2(x,y,t) = \frac{1}{2}|E_2(x,y)|\exp\{i(\omega_2 t - \phi_2(x,y))\} + cc \quad \textbf{(15)}$$

We will now carry out a *thought experiment*: We will consider that both object waves superpose and arrive at a "virtual" sensor which could resolve any time-dependent fast-oscillating interference fringes. Since we have retrieved the exact expressions for $E_1(x,y,t)$ and $E_2(x,y,t)$, we could easily simulate this *thought experiment*.

Please note that we do not need to consider the reference beams anymore, as they do not carry information about the object. They were helpful in the actual experiment only to retrieve the fields shown in Eq. 15.

As $E_1(x,y,t)$ and $E_2(x,y,t)$ have slightly different wavelengths, their superposition $E_{\text{obj}}(x,y) = E_1(x,y,t) + E_2(x,y,t)$ generates a so-called *beat wave* [2]. The intensity of this simulated beat is

$$I_{\text{obj}}(x,y) \propto |E_1(x,y) + E_2(x,y)|^2$$

$$= \frac{|E_1(x,y)|^2}{2} + \frac{|E_1(x,y)|^2}{2} + E_\Lambda(x,y) + \xi(x,y) \quad \textbf{(16)}$$

The two first addends correspond to a DC term, a static background illumination. The latter two terms correspond to the interferences and produce the time-dependent fringes. $E_\Lambda(x,y)$ denotes the slowly oscillating envelope that changes in time. This term has a temporal frequency $\Omega = |\omega_1 - \omega_2|$, which is called the *beat frequency* [2]. In contrast, $\xi(x,y)$ contains the beat waves with the high temporal frequencies (the carrier frequencies of the beat).

We can explicitly write the beat envelope by substituting Eq. 15 into Eq. 16,

$$E_\Lambda(x,y,t) = |E(x,y;\lambda_1)||E(x,y;\lambda_2)|\cos([\omega_1 - \omega_2]t + [\phi(x,y;\lambda_1) - \phi(x,y;\lambda_2)]) \quad \textbf{(17)}$$

One can then determine the *beat wavelength* using the following relationships:

$$\Lambda = \frac{2\pi c}{\Omega} = \frac{2\pi c}{|\omega_1 - \omega_2|} = \frac{2\pi c}{|\frac{2\pi c}{\lambda_1} - \frac{2\pi c}{\lambda_2}|} = \frac{\lambda_1\lambda_2}{|\lambda_1 - \lambda_2|} \quad \textbf{(18)}$$

Performing the calculations for $\xi(x,y)$, one find three terms with high temporal frequencies: $\omega_{12} = \omega_1 + \omega_2$, $\omega_{11} = 2\omega_1$, and $\omega_{22} = 2\omega_2$. These additional terms do not carry valuable information about the macroscopic object surface variation, as the corresponding wavelengths are roughly similar to the optical wavelengths, i.e., in the nanometer range: $\lambda_{12} = \lambda_1\lambda_2/|\lambda_1 + \lambda_2|$, $\lambda_{11} = \lambda_1/2$ and $\lambda_{22} = \lambda_2/2$. We shall neglect these terms in the following for our virtual beat wave.

So far, we have worked with our designed *thought experiment*. However, it should be emphasized that, in the real experiment, the two object waves indeed superpose and form a beat wave that arrives at the sensor, as in Eq. 16. Unfortunately, conventional sensors cannot resolve any of the time-dependent beat interferences (neither $E_\Lambda(x,y)$ nor $\xi(x,y)$). To give some rough estimation, let us consider the temporal beat frequency $\Omega = \omega_1 - \omega_2$. For $\lambda_1 = 850$ nm and $\lambda_2 = 850.02$ nm, we obtain $\Omega = 1.3 \times 10^9$ Hz. Conventional cameras have a presumably exposure time of around $10^{-3}$ seconds. If we integrate Eq. 17 average over the camera exposure time, we obtain an average intensity of zero (the fringes in $E_\Lambda(x,y)$ blur out). The same situation happens for the fast oscillating waves from $\xi(x,y;\lambda_1,\lambda_2)$.

We refer to the object beat $E_{\text{obj}}(x,y)$ as the "synthetic" beat in the sense that its time-dependent beat oscillations are

not naturally observed (besides being a physical process occurring in our actual single-shot experiment). As mentioned in section 3.2 from the main paper, the double-shot method recovers the optical fields $E(\lambda_1)$ and $E(\lambda_2)$ sequentially. In that case, the object fields are produced at different time and do not superpose in the actual experiment. The "synthetic" beat is then purely theoretical/simulated.

The beat envelope is commonly denoted as $E(\Lambda) \equiv E_\Lambda(x,y,t)$ and called the *synthetic wave*. Since E(Λ) changes over time, we should compute it at a fixed time (for example, at $t_0 = 0$). We can then rewrite Eq. 17 as

$$E(\Lambda) = |E(\lambda_1)||E(\lambda_2)|\cos(\phi(\lambda_1) - \phi(\lambda_2)) \tag{19}$$

Where $\phi(\Lambda) = \phi(\lambda_1) - \phi(\lambda_2)$ is referred to as the *synthetic phasemap*. For the previous example with $\Omega = 1.3 \times 10^9$ 1/s, we would get a synthetic wavelength $\Lambda \approx 3.6$ mm, though we could tune our lasers for different $\lambda_1$ and $\lambda_2$ to get multiple synthetic wavelengths. The importance of our *thought experiment* and the computational construction of the *synthetic wave* is the following:

*While the optical waves are susceptible to microscopic optical path length differences generated by the rough object surface, the synthetic wavelength is larger and less sensitive, providing us with a phase map that is not "speckled," i.e., not subject to random phase variations.*

An intuitive idea is provided in Section 2.1 of the main paper. Supp. fig. 5f shows the synthetic phase map which encodes the depth information of the object surface via Eq. 1 of the main paper. Moreover, supp. fig. 5e shows the square-root amplitude $|E(\Lambda)|^{1/2}$ of the synthetic wave. We plot the square-root amplitude of the synthetic wave to preserve the physical units of the electric field (W/m) and to see the clear correlation between $|E(\lambda_1)|$ and $|E(\lambda_2)|$ in supp. fig. 5. If two speckle points are correlated in $|E(\lambda_1)|$ and $|E(\lambda_2)|$, then we will see a bright point in $|E(\Lambda)|^{1/2} = |E(\lambda_1) \cdot E(\lambda_2)|^{1/2}$. However, this bright point will dim as the correlation between both fields is lost. In our experiments, $\lambda_1$ is only slightly different from $\lambda_2$ (with less than 0.02 nm of difference). Therefore, we observe a high spectral correlation between the speckles of $|E(\lambda_1)|$ and $|E(\lambda_1)|$. For our current experiments, we typically use $\Lambda = 1, 3, 10, 15, 30, 45, 50$ mm, in the order of magnitude of the depth of the objects we are measuring.

**Observation:** Another equivalent way to derive the (synthetic) interference term $E(\Lambda)$ is with the *wave mixing* formula [11] (see also Ch. 1 from [1]). In particular, the synthetic wave is given by the following *wave mixing* term:

$$\begin{aligned} E(\Lambda) &= \frac{1}{2} E(\lambda_1) \cdot E(\lambda_2)^* + cc \\ &= |E(\lambda_1)| \cdot |E(\lambda_2)| \cdot \cos(\phi(\lambda_1) - \phi(\lambda_2)) \end{aligned} \tag{20}$$

Eq. 7 is equivalent to the interference term from eq. 5. Although one can use both complementary theories to derive the synthetic beat wave[1], it should be emphasized that the wave mixing process does not happen "in reality" ( i.e., in our actual experiment), although we can perform the process on our computer. "In reality", wave mixing happens, e.g., when two (or more) optical waves propagate through non-linear crystals and generate another *actual* light wave at different frequencies (such as the second harmonic). In our experiment, $E(\Lambda)$ corresponds to the *envelope* of the beat wave between $E(\lambda_1)$ and $E(\lambda_2)$, which oscillates too fast to be resolved by our sensors (i.e., $E(\Lambda)$ is not an *actual* electromagnetic wave with wavelength Λ - it is only the amplitude modulation of two interfering waves).

## 3. Non-Line-of-Sight experiment.

Section 3.4 of the main paper explains the Non-Light-of-Sight (NLoS) experiment. To recap briefly, we used the object source (the end of an optical fiber that simultaneously emits light at $\lambda_1$ and $\lambda_2$) as a self-illuminating single-point object. This object was hidden behind a 220 grit ground glass diffuser. Direct imaging of the object with the camera was not possible due to the fairly strong scattering (see Fig. 7 from the main paper). We focused the camera on the rough surface of the diffuser and captured a single-shot image $I(x,y)$.

[1] The equivalent formulas 5 and 7 for the synthetic wave are represented in *real* notation, while the corresponding Eq. 2 of the main paper is expressed in *complex* notation. To be consistent with the derivations of this supp. mat., we understand that only the real part of the complex field should be taken (discarding the imaginary part from Eq. 2 of the main paper).

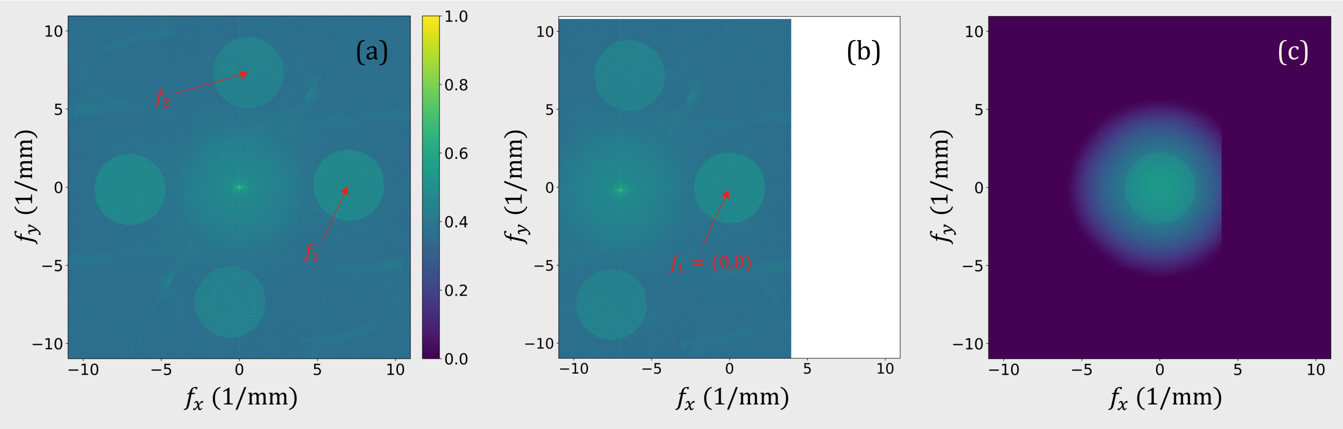


**Fig. 4.** (a) Fourier transform of the captured image $I(x,y)$. (b) Shifting the Fourier spectrum so that the carrier frequency $f_1$ corresponding to the horizontal reference beam is displaced to the center. (c) Applying a Gaussian filter to the shifted Fourier spectrum to uniformly remove any signals outside the region.

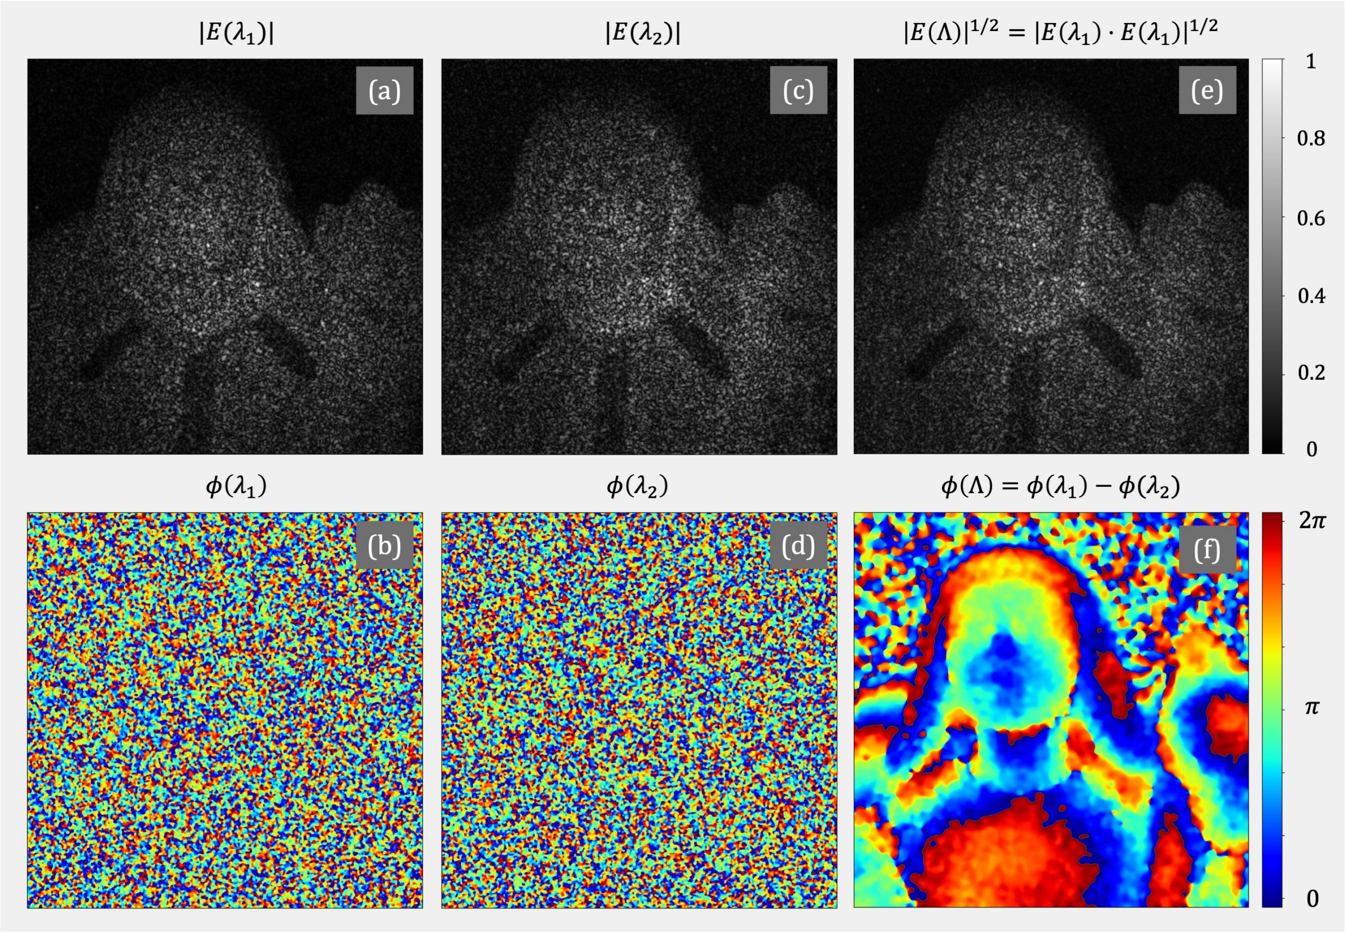


**Fig. 5.** (a) Amplitude and (b) phase of the object beam reflected by the object with wavelength $\lambda_1$. Similarly, (c) and (d) represent the amplitude and phase of the object beam reflected by the object with wavelength $\lambda_2$. Then, (e) and (f) show the calculated synthetic wave, $\Lambda$.

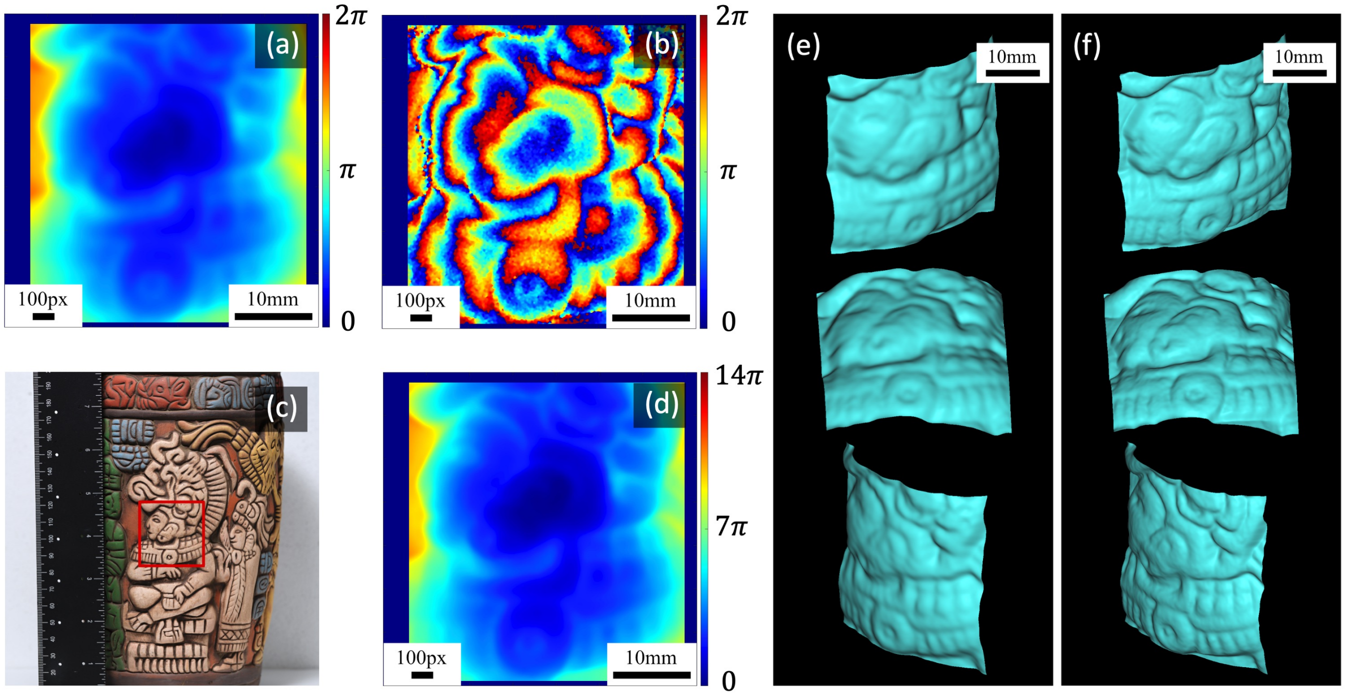


**Fig. 6.** Double-shot acquisition mode. The measured object is a clay pot approximately 20 cm in height. The camera FoV was cropped to about $40 \times 40$ mm$^2$: (a) Acquired synthetic phase map $\phi(\Lambda = 20\text{mm})$. (b) Wrapped phasemap $\phi(\Lambda = 3\text{mm})$. (c) Image of the small object with a window (red) showing the FoV. (d) Phasemap $\phi^{\text{unwrap}}(\Lambda = 3\text{mm})$, unwrapped with our multi-frequency unwrapping algorithm. (e) and (f) 3D model of the object calculated from $\phi(\Lambda = 20\text{mm})$ (e) and from unwrapped phasemap $\phi^{\text{unwrap}}(\Lambda = 3\text{mm})$.

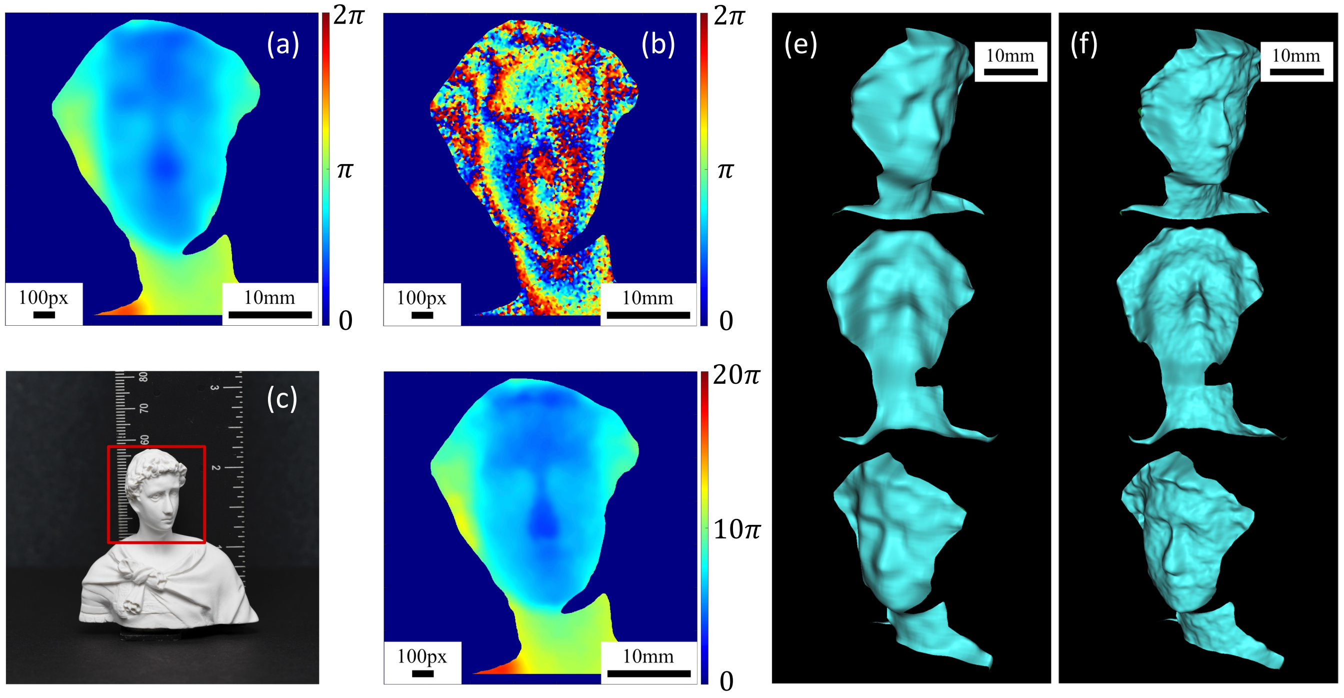


**Fig. 7.** Single-shot acquisition mode. The measured object is a plaster bust of approximately 6 cm in height. (a) Acquired synthetic phase map $\phi(\Lambda = 50\text{mm})$. (b) Wrapped phasemap $\phi(\Lambda = 5\text{mm})$. (c) Image of the small object with a window (red) showing the FoV. (d) Phasemap $\phi^{\text{unwrap}}(\Lambda = 5\text{mm})$, unwrapped with our multi-frequency unwrapping algorithm. (e) and (f) 3D model of the object calculated from $\phi(\Lambda = 50\text{mm})$ (e), and from unwrapped phasemap $\phi^{\text{unwrap}}(\Lambda = 5\text{mm})$ (f).

Using our proposed method (section 2.2 from the main paper), we recovered the synthetic field $E(\Lambda = 1\text{mm})$, which can be now interpreted as a *"synthetic hologram"* of the object. This is because $E(\Lambda = 1\text{mm})$ is not the field distribution directly on the object surface but rather the propagated field (since the camera was focused at the diffuser location and the object was placed further away). Similar to [11], we can now use the Angular Spectrum Method [10] to backpropagate the field into the hidden volume to obtain a reconstruction of the object.

As it was done by the authors of [11], we now want to determine the theoretical resolution of our object reconstruction by calculating the diffraction limit of our system at the synthetic wavelength. According to the Abbe diffraction limit (see [2] and [11]), the minimal laterally resolvable distance in the hidden volume is given by $\delta x = \frac{\Lambda}{2\text{NA}}$. In our case, the aperture is defined by the observable region on the diffuser (with a diameter of about $D = 66$ mm). With the object standoff distance of $z = 300$ mm, the numerical aperture calculates to $\text{NA} = n\sin(\theta) \approx \tan(\theta) = \frac{D/2}{z} \approx 33\text{mm}/300\text{mm} = 0.11$ and hence, the theoretical lateral resolution to $\delta x = \frac{\Lambda}{2\text{NA}} \approx \frac{1\text{mm}}{2 \cdot 0.11} \approx 4.55\text{mm}$. It can be seen in Fig. 7c of the main paper that this theoretical calculation roughly matches the radius of the reconstructed object (about $\delta_x^{\text{exp}} \approx 5$ mm radius), meaning that our shown NLoS measurement reached diffraction-limited performance at the synthetic wavelength.

## 4. Analysis and further results.

### A. Results using the multifrequency unwrapping algorithm.

In the sec. 2.2 and 2.3 of the main paper, we show the results of the double-shot and single-shot methods using our multifrequency unwrapping algorithm (see Figs. 3-4 in the main paper). In this section, we show additional results to demonstrate the versatility of our approach.

For the double-shot method, we imaged a small clay pot with fine 3D reliefs (see supp. fig. 6c). Supp. fig. 6a displays an unwrapped synthetic phasemap of the object acquired at a large synthetic wavelength of $\Lambda = 20$ mm. Supp. fig. 6b shows a wrapped synthetic phasemap acquired at $\Lambda = 3$ mm.

Using our multifrequency unwrapping algorithm, one can find the unwrapped synthetic phasemap $\phi^{\text{unwrap}}(\Lambda = 3\text{mm})$ using $\phi(\Lambda = 20\text{mm})$ as the guidance phasemap. Supp. figs. 6 e-f show the object's 3D model calculated from $\phi(\Lambda = 20\text{mm})$ and $\phi^{\text{unwrap}}(\Lambda = 3\text{mm})$, respectively, via Eq. 1 of the main paper. As can be seen, our method is able to impressively resolve the fine imprinted details of the clay pot in 3D.

In addition, we show similar results for the single-shot method to image a small bust figure (see supp. fig. 7c). In this case, the large wavelength is $\Lambda = 50$ mm, and the smaller one, $\Lambda = 5$ mm.

### B. Deep Learning unwrapping algorithm.

To exploit the main feature of our novel camera, we need to unwrap the synthetic phasemaps from a single shot image. Conventional single-shot unwrapping algorithms (such

as those predefined in Matlab or Python) fail to unwrap our phasemaps due to their geometric complexity and the relatively large noise level. For that reason, we have built a Deep-Learning-based unwrapping algorithm. Compared to other state-of-the-art phase unwrapping procedures [12, 13], our approach is specifically tailored to our data structure.

As briefly discussed in the main paper, our approach defines a Convolutional Neural Network (CNN) with an encoder-decoder structure [14–16]. Inspired by the work from Perera *et al.* [17], we also added a Long Short-Term Memory (LSTM) module into our network. The LSTM modules are commonly used in Recurrent Neural Networks to solve the so-called "vanishing gradient" problem [18, 19]. Nevertheless, it is also becoming a powerful tool in CNNs to learn the spatial relations between local features [20, 21]. In phase unwrapping problems, these spatial relations between local features are essential to identify the phase jumps.

The LSTM module was added between the encoder and decoder networks: It takes in the local features from the encoded image and provides their local spatial relations to the decoder network. The structure of the network is shown in supp. fig. 8. One can observe that each layer from the encoder is concatenated with a corresponding decoder layer [16, 22]. This concatenation provides information to the decoder that was otherwise lost during downsampling (or encoding phase). The network predicts more accurately if we combine the extracted features (from the encoder) with the original values (given through the concatenation).

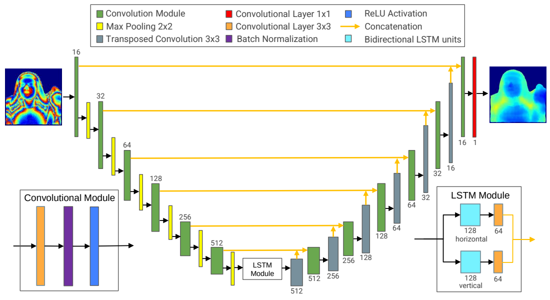


**Fig. 8.** Architecture of the Deep Learning algorithm.

The training dataset employs both experimental and simulated data. For the experimental part, we use wrapped synthetic phasemaps directly obtained from our camera. To build the input-output pairs consisting of wrapped and unwrapped phasemaps, we use our multifrequency unwrapping algorithm.

For the simulated data, we first created realistic 3D models of common objects using *Mitsuba 3* [23]. Given the depth information $D(x,y) = z$ from *Mitsuba*, one can quickly generate unwrapped phasemaps $\phi^{\text{unwrap}}(x,y;\Lambda)$ for different synthetic wavelengths $\Lambda$ using the Eq. 1 of the main paper. Eventually, phase wrapping is performed using the *modulus* operation. To have more realistic simulated data, we have introduced a certain noise level. We have added Gaussian noise ($\mu = 0, \sigma = \pi/6$) to each wrapped phasemap pixel that randomly reduces or increases the pixel value.

We had 22 pairs of wrap-unwrap phasemaps for real objects at a relatively small synthetic wavelength (around 3-10 mm). We increased this experimental dataset to 66 by including rigid transformations of the phasemaps (reflection, rotation, and translations). In addition, we developed 21 pairs of wrap-unwrap phasemaps for simulated objects from *Mitsuba*. Considering the rigid transformations of the simulated phasemaps, different noise levels, and different synthetic wavelengths, we increased the simulated dataset size up to 1512. The training dataset (with real and simulated data) had 1578 data. Supp. fig. 9 shows one of the simulated pairs of data from the training dataset: A wrapped phasemap that serves as input and its associated nicely unwrapped phasemap corresponding to its output.

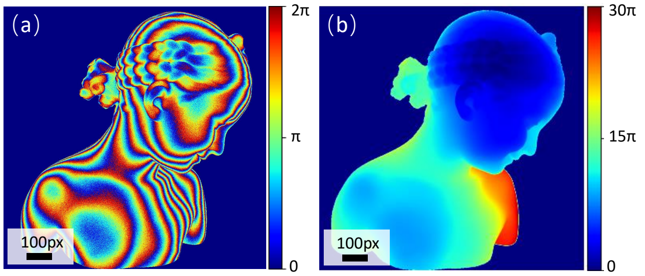


**Fig. 9.** Simulated data for the training of the Deep Learning unwrapping algorithm. We employed *Mitsuba* [23] to simulate realistic 3D objects. (a) Input: Wrapped noisy phasemap. (b) Output: Unwrapped phasemap.

The loss function for our network measures the mean squared error (MSE) between the ground truth unwrapped phase map and the predicted phase map. During the training process, the parameters of the CNN are optimized so that the model produces accurate unwrapped output phase maps out of the wrapped input phase maps. Once the model is trained, we test the model's performance using the wrapped phasemaps of new objects. We emphasize again that the unwrapping model has neither seen the test data phasemaps before nor any other measurements of the test objects (e.g., phasemaps at different wavelengths, measurements of the same object taken from a different perspective, etc.).

To improve the network's accuracy, we should also mention that we divided the training according to different synthetic wavelengths (relatively small wavelengths between 3-10 mm, or rather large wavelengths around 30-45 mm). Besides the result provided in the main paper in Fig. 7, we provide in supp. fig. 10 another result for the measurement of a bust.

## C. Smoothing parameters for shown images.

For the sake of transparency and reproducibility, we provide below the smoothing parameters we have employed for our results (both in the main paper and the Supp. Mat.).

- **Fig. 3 (a)** of the main paper. We first applied a 2D Gaussian filter on the complex synthetic field $E(\Lambda = 45\text{mm})$ with $\sigma = 4$ and a kernel size $K = 20 \times 20$. Then, we employed the median filter on the phase map, with a kernel size $K = 21 \times 21$ pixels. Finally, we used a

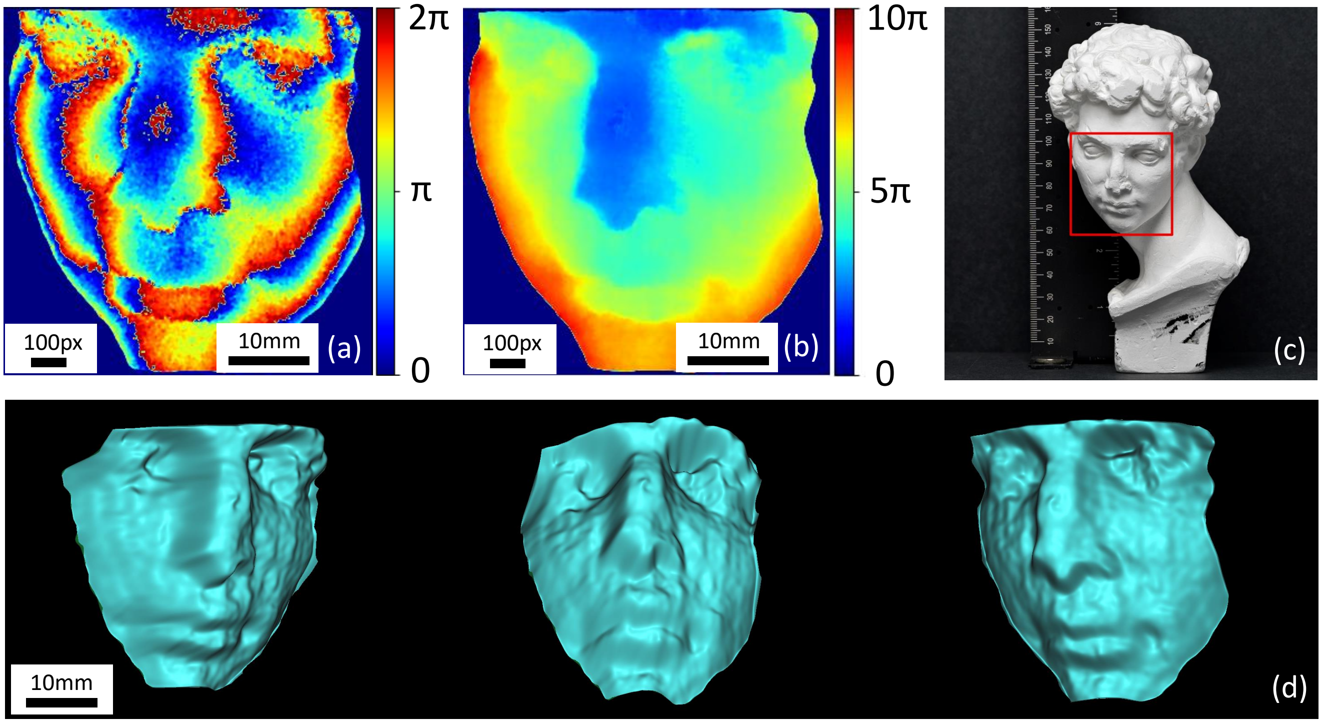


**Fig. 10.** Single-shot deep learning-based phase unwrapping method. (a) Wrapped phase map $\phi(\Lambda = 10\text{mm})$. (b) Unwrapped phase map predicted by the neural network approach. (c) Image of the small object with a window (red) showing FoV. (d) 3D model of the object calculated from unwrapped phasemap $\phi^{\text{unwrap}}(\Lambda = 10\text{mm})$.

strong Gaussian filter on the phase map with $\sigma = 30$ and $K = 121 \times 121$ pixels.

- **Fig. 3 (d)** of the main paper. We first applied a 2D Gaussian filter on the complex synthetic field $E(\Lambda = 10\text{mm})$ with $\sigma = 4$ and $K = 20 \times 20$ pixels. Then, we employed the median filter on the phase map with $K = 41 \times 41$ pixels. Finally, we used the Gaussian filter on the unwrapped phase map with $\sigma = 9$ and $K = 37 \times 37$ pixels.

- **Fig. 4 (a)** of the main paper. We first applied a 2D Gaussian filter on the complex synthetic field $E(\Lambda = 50\text{mm})$ with $\sigma = 4$ and $K = 20 \times 20$ pixels. Then, we employed the median filter on the phase map with $K = 21 \times 21$ pixels. Finally, we used the Gaussian filter on the phase map with $\sigma = 40$ and $K = 161 \times 161$ pixels.

- **Fig. 4 (d)** of the main paper. We first applied a 2D Gaussian filter on the complex synthetic field $E(\Lambda = 10\text{mm})$ with $\sigma = 10$ and $K = 10 \times 10$ pixels. Then, we employed the median filter on the phase map with $K = 41 \times 41$ pixels. Finally, we used the Gaussian filter on the unwrapped phasemap with $\sigma = 9$ and $K = 37 \times 37$ pixels.

- **Fig. 5 (b) and (d)** of the main paper. We first applied a 2D Gaussian filter on the complex synthetic field $E(\Lambda = 30\text{mm})$ with $\sigma = 10$ and $K = 60 \times 60$ pixels. Then, we employed the median filter on the phase map with $K = 21 \times 21$ pixels. We additionally applied a bilateral filter using the predefined Matlab function *imbilatfilt* using 1 degree of smoothing a $\sigma = 20$. Finally, we used the Gaussian filter on the phase map with $\sigma = 20$ and $K = 81 \times 81$ pixels.

- **Supp. fig. 6 (a)**. We first applied a 2D Gaussian filter on the complex synthetic field $E(\Lambda = 20\text{mm})$ with $\sigma = 4$ and $K = 20 \times 20$ pixels. Then, we employed the median filter on the phase map with $K = 21 \times 21$ pixels. Finally, we used the Gaussian filter on the phase map with $\sigma = 20$ and $K = 81 \times 81$ pixels.

- **Supp. fig. 6 (d)**. We first applied a 2D Gaussian filter on the complex synthetic field $E(\Lambda = 3\text{mm})$ with $\sigma = 4$ and $K = 20 \times 20$ pixels. Then, we employed the median filter on the phase map with $K = 41 \times 41$ pixels. Finally, we used the Gaussian filter on the unwrapped phase map with $\sigma = 9$ and $K = 37 \times 37$ pixels.

- **Supp. fig. 7 (a)**. We first applied a 2D Gaussian filter on the complex synthetic field $E(\Lambda = 50\text{mm})$ with $\sigma = 4$ and $K = 20 \times 20$ pixels. Then, we employed the median filter on the phase map with $K = 21 \times 21$ pixels. Finally, we used the Gaussian filter on the phase map with $\sigma = 40$ and $K = 161 \times 161$ pixels.

- **Supp. fig. 7 (d)**. We first applied a 2D Gaussian filter on the complex synthetic field $E(\Lambda = 5\text{mm})$ with $\sigma = 2$ and $K = 10 \times 10$ pixels. Then, we employed the median filter on the phase map with $K = 41 \times 41$ pixels. Finally, we used the Gaussian filter on the unwrapped phase map with $\sigma = 9$ and $K = 37 \times 37$ pixels.

- **Fig. 6b of the paper and supp. fig. 10b**. We first

applied a 2D Gaussian filter on the complex synthetic field $E(\Lambda = 10\text{mm})$ with $\sigma = 7$ and $K = 40 \times 40$ pixels. Then, we employed the median filter on the unwrapped phase map with $K = 21 \times 21$ pixels. Finally, we used the Gaussian filter on the unwrapped phase map with $\sigma = 10$ and $K = 41 \times 41$ pixels.

## 5. Bibliography.


[1] Geoffrey New. *Introduction to nonlinear optics*. Cambridge University Press, 2011.

[2] Eugene Hecht. *Optics, 5e*. Pearson Education India, 2002.

[3] Mitsuo Takeda, Hideki Ina, and Seiji Kobayashi. Fourier-transform method of fringe-pattern analysis for computer-based topography and interferometry. *JosA*, 72(1):156–160, 1982.

[4] Mitsuo Takeda and Seiji Kobayashi. Lateral aberration measurements with a digital talbot interferometer. *Applied Optics*, 23(11):1760–1764, 1984.

[5] Nicolas Verrier and Michael Atlan. Off-axis digital hologram reconstruction: some practical considerations. *Applied optics*, 50(34):H136–H146, 2011.

[6] Tatsuki Tahara and Yasuhiko Arai. Multiwavelength off-axis digital holography with an angle of more than 40 degrees and no beam combiner to generate interference light. *Applied optics*, 56(13):F200–F204, 2017.

[7] Venugopal Srinivasan, Hsin-Chu Liu, and Maurice Halioua. Automated phase-measuring profilometry of 3-d diffuse objects. *Applied optics*, 23(18):3105–3108, 1984.

[8] Mitsuo Takeda and Kazuhiro Mutoh. Fourier transform profilometry for the automatic measurement of 3-d object shapes. *Applied optics*, 22(24):3977–3982, 1983.

[9] Peter De Groot. Interferometric laser profilometer for rough surfaces. *Optics letters*, 16(6): 357–359, 1991.

[10] Joseph W Goodman. Introduction to fourier optics. 3rd. *Roberts and Company Publishers*, 3, 2005.

[11] Florian Willomitzer, Prasanna V Rangarajan, Fengqiang Li, Muralidhar M Balaji, Marc P Christensen, and Oliver Cossairt. Fast non-line-of-sight imaging with high-resolution and wide field of view using synthetic wavelength holography. *Nature communications*, 12(1): 1–11, 2021.

[12] Shuochen Su, Felix Heide, Gordon Wetzstein, and Wolfgang Heidrich. Deep end-to-end time-of-flight imaging. In *Proceedings of the IEEE Conference on Computer Vision and Pattern Recognition*, pages 6383–6392, 2018.

[13] Seung-Hwan Baek, Noah Walsh, Ilya Chugunov, Zheng Shi, and Felix Heide. Centimeter-wave free-space neural time-of-flight imaging. *ACM Transactions on Graphics (TOG)*, 2022.

[14] Olaf Ronneberger, Philipp Fischer, and Thomas Brox. U-net: Convolutional networks for biomedical image segmentation. In *International Conference on Medical image computing and computer-assisted intervention*, pages 234–241. Springer, 2015.

[15] Jeremy Watt, Reza Borhani, and Aggelos K Katsaggelos. *Machine learning refined: Foundations, algorithms, and applications*. Cambridge University Press, 2020.

[16] Rajalingappaa Shanmugamani. *Deep Learning for Computer Vision: Expert techniques to train advanced neural networks using TensorFlow and Keras*. Packt Publishing Ltd, 2018.

[17] Malsha V Perera and Ashwin De Silva. A joint convolutional and spatial quad-directional lstm network for phase unwrapping. In *ICASSP 2021-2021 IEEE International Conference on Acoustics, Speech and Signal Processing (ICASSP)*, pages 4055–4059. IEEE, 2021.

[18] Sepp Hochreiter and J"urgen Schmidhuber. Long short-term memory. *Neural computation*, 9(8):1735–1780, 1997.

[19] Sepp Hochreiter. The vanishing gradient problem during learning recurrent neural nets and problem solutions. *International Journal of Uncertainty, Fuzziness and Knowledge-Based Systems*, 6(02):107–116, 1998.

[20] Jawadul H Bappy, Cody Simons, Lakshmanan Nataraj, BS Manjunath, and Amit K Roy-Chowdhury. Hybrid lstm and encoder–decoder architecture for detection of image forgeries. *IEEE Transactions on Image Processing*, 28(7):3286–3300, 2019.

[21] Fan Xu, Haoyu Ma, Junxiao Sun, Rui Wu, Xu Liu, and Youyong Kong. Lstm multi-modal unet for brain tumor segmentation. In *2019 IEEE 4th international conference on image, vision and computing (ICIVC)*, pages 236–240. IEEE, 2019.

[22] Rajalingappaa Shanmugamani. *Deep Learning for Computer Vision: Expert techniques to train advanced neural networks using TensorFlow and Keras*. Packt Publishing Ltd, 2018.

[23] Wenzel Jakob. Mitsuba renderer, 2010. http://www.mitsuba-renderer.org.
